# Supplementary material for: Building connections: How scientists meet each other during a conference
Source: arXiv:1901.01182 ancillary file (2019-01-07)
Supplement: Supplementary file 1 [file Supplementary_information.pdf]

# Supplementary information
# for
# Building connections: How scientists meet each other during a conference

Mathieu Génois*
*CNRS, CPT, Aix Marseille Univ, Université de Toulon, Marseille, France and*
*GESIS, Leibniz Institute for the Social Sciences, Köln, Germany*

Maria Zens, Clemens Lechner, and Beatrice Rammstedt
*GESIS, Leibniz Institute for the Social Sciences, Köln, Germany*

Markus Strohmaier
*GESIS, Leibniz Institute for the Social Sciences, Köln, Germany and*
*RWTH Aachen University*
(Dated: November 8, 2018)

* mathieu.genois@gesis.org

# I. SOCIODEMOGRAPHIC FEATURES

Table I summarises the numbers associated with each socio-demographic dimension for both datasets.

| | **WS16** | | | **ICCSS17** | | |
|---|---|---|---|---|---|---|
| **Category** | **Label** | $N$ | % | **Label** | $N$ | % |
| **Age range** | < 30 | 53 | 46.1 % | < 30 | 55 | 27.6 % |
| | 30 to 39 | 46 | 40.0 % | 30 to 39 | 98 | 49.2 % |
| | > 40 | 16 | 13.9 % | 40 to 49 | 31 | 15.6 % |
| | | | | > 50 | 15 | 7.54 % |
| **Gender** | M | 66 | 57.4 % | M | 138 | 69.3 % |
| | F | 49 | 42.6 % | F | 61 | 30.7 % |
| **Country of residence** | Country 1 | 63 | 56.8 % | Country 1 | 55 | 27.5 % |
| | Other | 48 | 43.2 % | Country 2 | 42 | 21.0 % |
| | | | | Country 3 | 18 | 9.00 % |
| | | | | Country 4 | 10 | 5.00 % |
| | | | | Other | 65 | 32.5 % |
| **Mothertongue** | Language 1 | 47 | 43.5 % | Language 1 | 49 | 25.7 % |
| | Language 2 | 18 | 16.7 % | Language 2 | 43 | 22.5 % |
| | Other | 43 | 39.8 % | Language 3 | 21 | 11.0 % |
| | | | | Language 4 | 15 | 7.85 % |
| | | | | Language 5 | 10 | 5.24 % |
| | | | | Other | 53 | 27.7 % |
| **Academic status** | Bachelor Student | 9 | 8.3 % | | | |
| | Master Student | 18 | 16.7 % | Master/Bachelor | 16 | 8.12 % |
| | PhD | 33 | 30.6 % | PhD | 63 | 32.0 % |
| | Postdoc | 24 | 22.2 % | Postdoc | 45 | 22.8 % |
| | Assist./Assoc. Res. | 8 | 7.4 % | Junior/Assist. Pr. | 29 | 14.7 % |
| | Professor | 12 | 11.1 % | Assoc./Full Pr. | 30 | 15.2 % |
| | Other | 4 | 3.7 % | Other (Industry/Staff) | 14 | 7.11 % |
| **Academic background** | Social sciences, Humanities, Political science | 50 | 45.4 % | Social/Political/Behavioural Sciences | 61 | 30.8 % |
| | Computer science, Information science | 39 | 35.4 % | Computer/Information Science | 72 | 36.4 % |
| | Physics, Mathematics, Statistics | 13 | 11.8 % | Math/Physics/Biology | 48 | 24.2 % |
| | Media, Communication, Other | 8 | 7.3 % | Media/Communication/Linguistics | 9 | 4.55 % |
| | | | | Others | 8 | 4.04 % |
| **Role** | Poster | 43 | 37.7 % | Poster | 44 | 21.9 % |
| | Speaker | 12 | 10.5 % | Speaker | 92 | 45.8 % |
| | Participation only | 43 | 37.7 % | Participation only | 50 | 24.9 % |
| | Staff | 16 | 14.0 % | Staff | 15 | 7.46 % |
| **Previous Participation** | Yes | 49 | 43.0 % | Yes | 70 | 34.7 % |
| | No | 65 | 57.0 % | No | 132 | 65.3 % |

TABLE I. **Socio-demographics.**

## II. GENERAL FEATURES OF THE CONTACT DATA

In this section we describe the general features of both the aggregated contact network and the temporal contact activity. The aggregated network is defined as the following:

- there exists a link between two individuals $i$ and $j$ if they have been at least once in contact during the study;
- each link $(i, j)$ has a weight $w_{ij}$ that describes the intensity of the interaction between $i$ and $j$; this weight is defined as the cumulative duration of contact between $i$ and $j$, *i.e.* the total time these two individuals have been in contact during the study.

All the following results are computed on the complete populations for which we have contact data (138 for WS16, 274 for ICCSS17).

### A. Contact activity

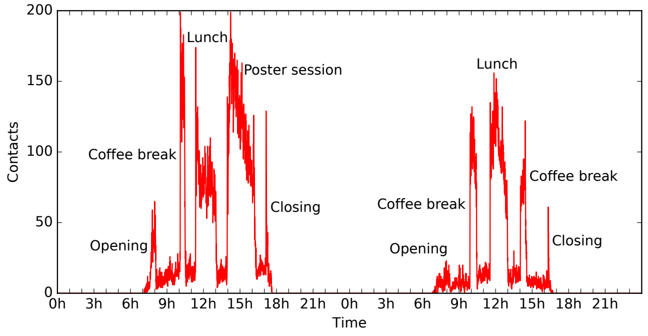


(a) **WS16**

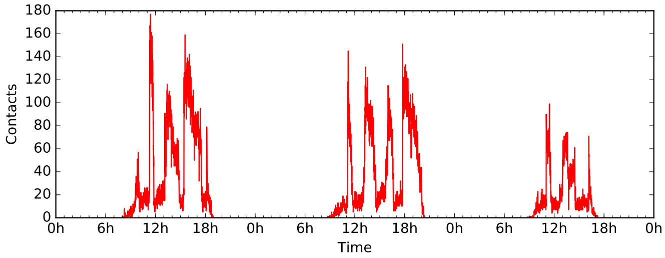


(b) **ICCSS17**

| Activity | Time | Period |
|---|---|---|
| | | ***First day*** |
| High | 07:00 | Opening of the conference |
| Low | 08:00 | First morning talk session |
| High | 10:00 | Morning coffee break |
| Low | 10:30 | Second morning talk session |
| High | 11:30 | Lunch |
| Low | 13:00 | First afternoon talk session |
| High | 14:00 | Poster Session |
| Low | 16:00 | Second afternoon talk session |
| High | 17:00 | Closing |
| | | ***Second day*** |
| Low | 07:00 | Opening & First morning talk session |
| High | 10:00 | Morning coffee break |
| Low | 10:30 | Second morning talk session |
| High | 11:30 | Lunch |
| Low | 13:00 | First afternoon talk session |
| High | 14:00 | Afternoon coffee break |
| Low | 14:30 | Second afternoon talk session |
| High | 16:30 | Closing of the conference |

(c) **Activity periods — WS16.**

FIG. 1. **Contact activity.** At each time $t$ we consider the number of contacts occurring in the whole system. For the WS16 case, the periods of high contact activity are annotated in the graph and reported in the Table.

We show on Figure II A the number of contacts occurring at each time step $t$, in which the days of the conferences are clearly separated. The contact activity is far from constant across time. The curves show alternating periods of very low and very high contact activity. Each window can thus be labelled according to the program of the conference without any ambiguity (Table 1c).

### B. Density, Degree & Strength

The density $\rho$ is defined as the ratio between the number of links in the aggregated network and the total number of possible links in the same network. Both networks are quite dense, ($\rho = 0.793$ for WS16, $\rho = 0.507$ for ICCSS17). For WS16, it is in fact close to a fully connected network. This is probably due to the fact that 1) we have an almost complete coverage of the venue, and 2) that the crowd was rather small and confined in a small venue, which favours proximity interactions.

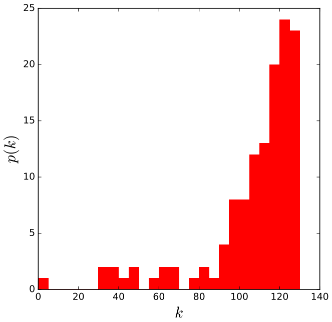


(a) **Degree — WS16.**

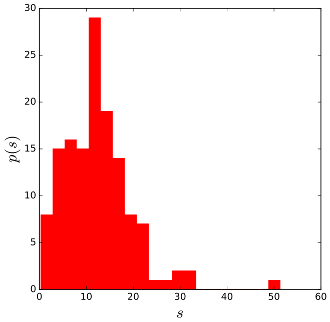


(b) **Strength — WS16.**

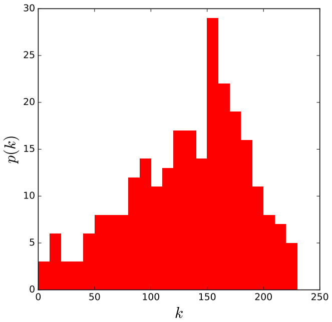


(c) **Degree — ICCSS17.**

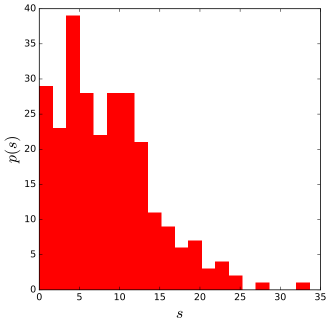


(d) **Strength — ICCSS17.**

FIG. 2. **Distributions of connectivity features.** We plot the distributions of the degree, *i.e.* the number of persons with whom each individual has been in contact at least once, and strength, *i.e.* the total time spent interacting. Strength is measured in number of hours.

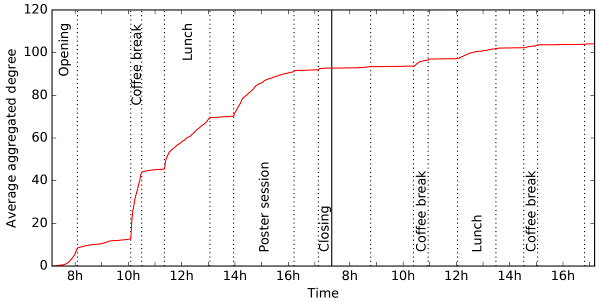


(a) **Degree — WS16.**

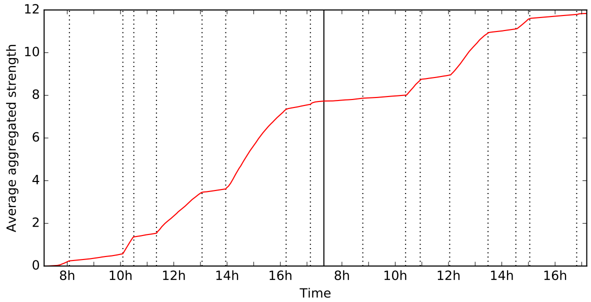


(b) **Strength — WS16.**

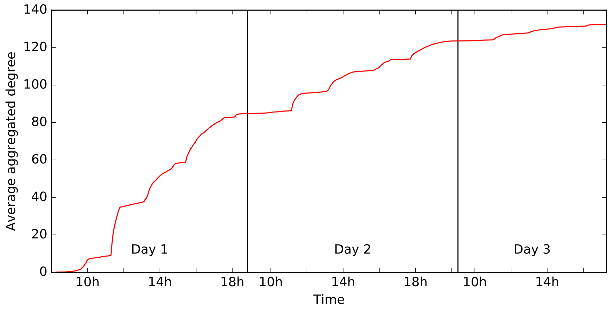


(c) **Degree — ICCSS17.**

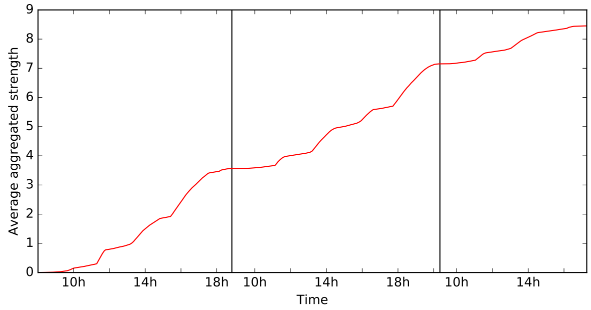


(d) **Strength — ICCSS17.**

FIG. 3. **Growths of connectivity features — WS16.** We compute the growth of the average degree and strength as we aggregate the network through time. The night has been removed, and is indicated by the vertical solid line. For the WS16 case, limits between the different activity periods are indicated by the vertical dotted lines. High activity periods are labeled.

The degree $k$ of a node of the network is defined as the number of nodes with which it is connected, *i.e.* the number of persons with whom each individual has been in contact at least once during the conference. In both cases the degree distribution of the aggregated network is skewed towards high degrees (Figs. 2a & 2c). This is a direct consequence from the high density of the network.

The strength $s$ of a node is defined as the sum of the weights of all the links attached to this node. In this case, link weights are set to the total time spent in contact. The stregnth is therefore the total time an individual has spent interacting with other individuals. Contrary to the degree distributions, the strength distributions (Figs. 2b & 2d) show a usual “log-normal-like” shape, with sharp increase from 0 to its peak at a relatively low strength, and a rather stretched tail towards high values of strengths. This indicates that even if nodes are almost all connected to each other, they do not interact with the same intensity. The whole range of behaviours, from weakly interacting to strongly interacting, exists, the most likely being an intermediate level of interaction.

On the growth of the average degree (Figs. 3a & 3c), we see that the average degree saturates as we aggregate the network through time. It is also worth noticing that the periods found in the activity (Fig. II A) are also found in the degree growth. Fast growth windows, corresponding to breaks, alternate with slow growth windows, corresponding to talk sessions. Both curves start with an exponential growth, and evolve towards a typical exponential saturation. Overall, during the first day of the conference the average degree reaches a very high value and starts saturating. This indicates that most individuals have met the majority of the persons they will meet at the end of the first day.

As for the average degree, the growth of the average strength (Figs. 3b & 3d) shows clearly the alternating between low interaction and high interaction periods, in two different regimes marked by two different rates of growth. However, the strength does not show any sign of saturation: people keep on interacting at the same rate during the whole conference.

## C. Temporal features

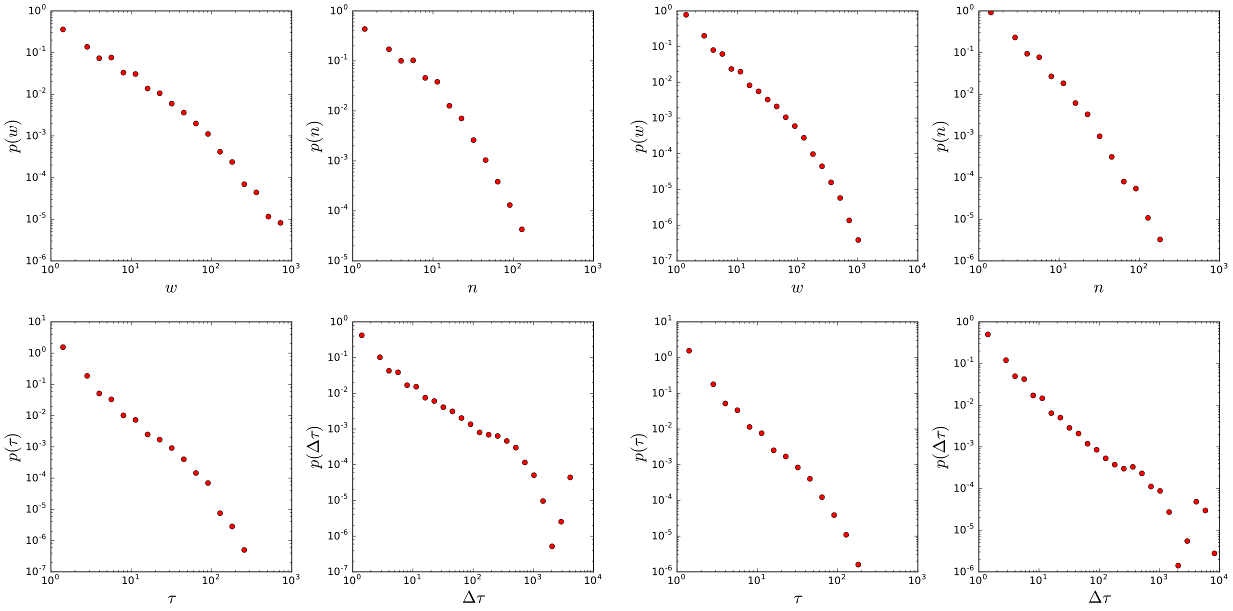


(a) **WS16.**

(b) **ICCSS17.**

FIG. 4. **Temporal features of the network.** These plots show the distributions of link weights $w$ (total contact duration between two nodes), number of contacts $n$ per link, contact durations $\tau$ and intercontact durations $\Delta\tau$.

We define an interaction event as a continuous succession of contacts. An interaction event thus has a duration $\tau$. The weight $w$ of a link is defined as the sum of the durations of the interactions occurring between the two individuals. On each link, interaction events are separated by inter event periods, which durations are noted $\Delta\tau$. The number of event for each link is noted $n$.

The distributions of these quantities are standard measures for this kind of physical proximity experiment. They always follow the same broad, power law-like distributions. We verify (Fig. 4) that it is also the case for these studies.

## III. GROUP HETEROGENITIES IN CONNECTIVITY

Figures 5 & 6 detail the heterogeneities in degree and strength between groups per day.

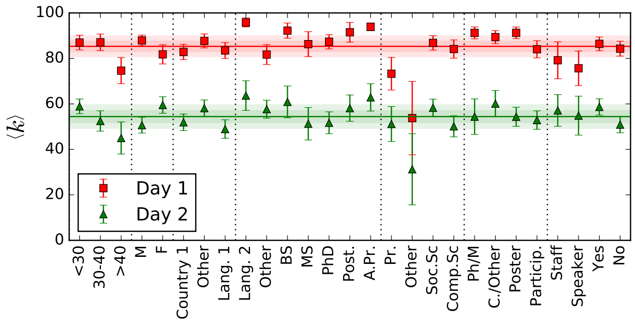


(a) **WS16**

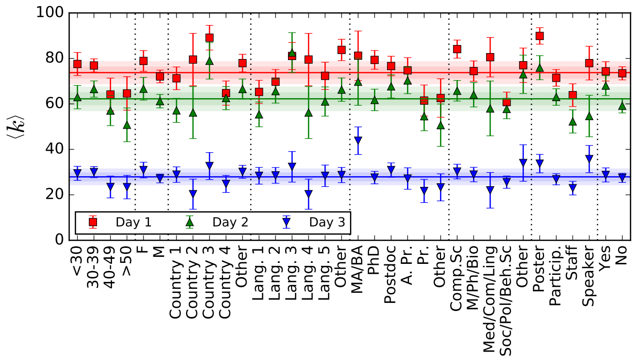


(b) **ICCSS17**

FIG. 5. **Average degree in each group, per day.** For each group we compute the average degree if the individuals, for each day. The error bar shows the standard error on the measure of this average degree. The solid colored line and colored regions show the overall average value for all nodes, with one and two standard deviations.

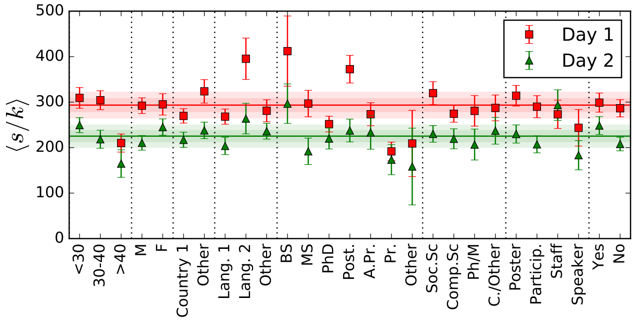


(a) **WS16**

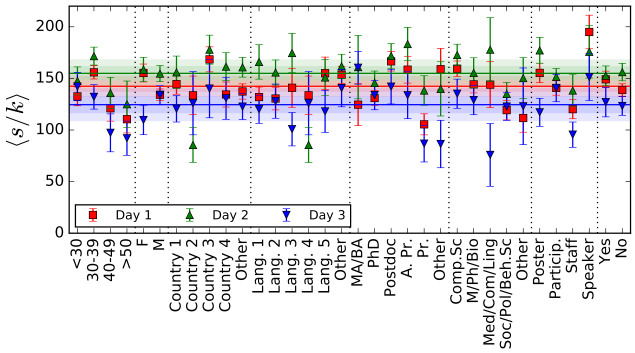


(b) **ICCSS17**

FIG. 6. **Average individual interaction duration in each group, per day.** For each group we compute the average individual interaction duration of the individuals, for each day. The durations are meausred in seconds. The error bar shows the standard error on the measure of this average degree. The solid colored line and colored regions show the overall average value for all nodes, with one and two standard deviations.

## IV. MIXING, HOMOPHILY AND AVOIDANCE BEHAVIOURS

**description figures**
Deviations fall into three categories:

- specific to a dataset and one or several randomisation;
- valid across randomisations for one dataset;
- valid for all randomisations and both datasets.

We present the results in Table II, both for significant deviations and deviations that are greater than 3 standard deviations but not significant under the corrections. For Age, we see that overall we tend to have homophily between younger participants both in connectivity and interactivity, while older participants tend to avoid each other. For Gender we see almost no signal, except for two contradictory cases. Country and Language both show a clear homophily between participants. For Acdemic status, it appears that non permanent connect and interact more, and that Professors and Others connect and interact less, especially with them. Some Disciplines show homophily, notably Computer Science and Social Sciences, furthermore these two seem to connect less. Some Roles are clearly homphilic, such as Staff in WS16, and Speakers and Poster presenters in ICCSS17.

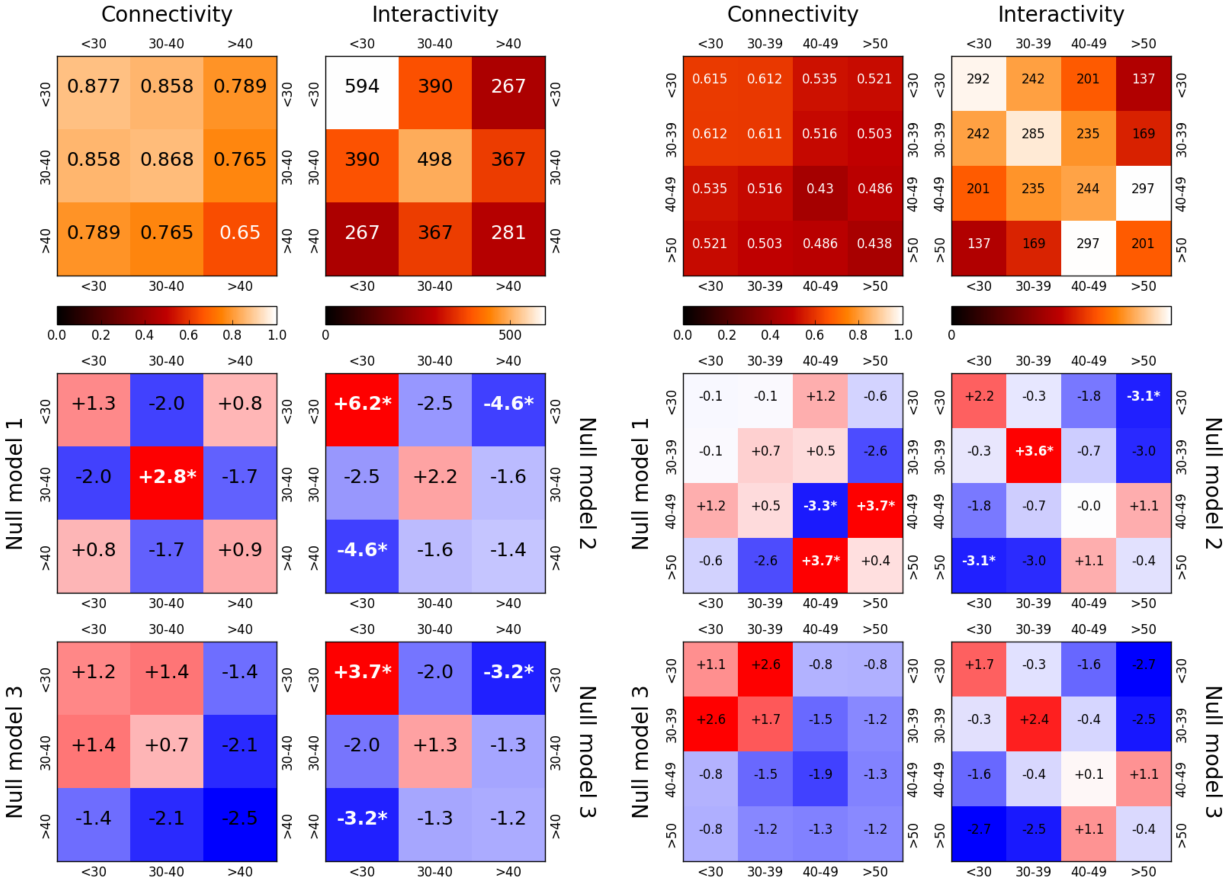


(a) **WS16** (b) **ICCSS17**

FIG. 7. **Contact matrices for age group.** We compute for each conference the contact matrix in connectivity (*i.e.* link density) and interactivity (*i.e.* average total contact duration) considering the age group (top row). We then test the statistical significance of the values of the contact matrices by performing three different null models: P[**k**] (Null model 1), P[$p(\mathbf{w})$] (Null model 2) and P[**iso**(**g**)] (Null model 3). Positive deviations are in red and negative deviations in blue. Deviations marked in white with a star are significant under $p < 0.01$ (taking into account a Bonferroni correction).

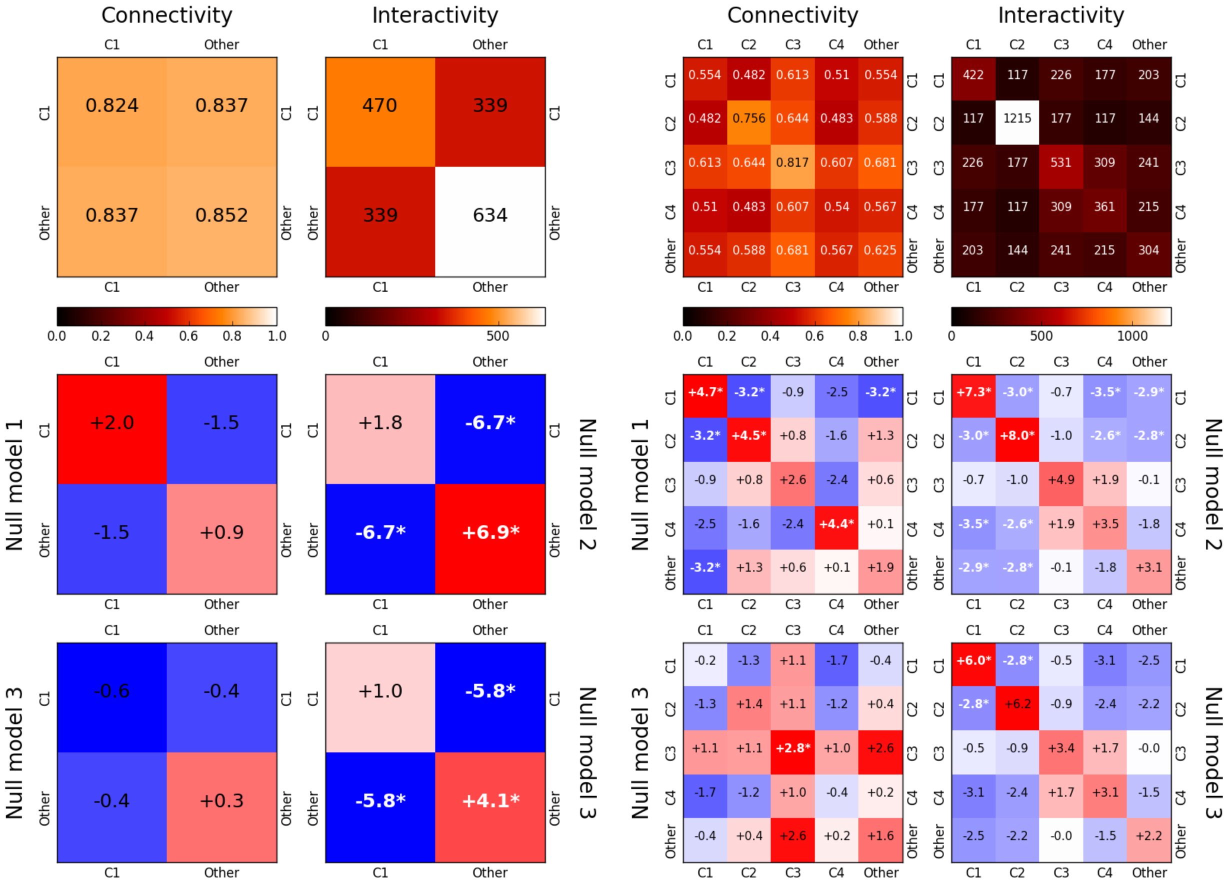


(a) **WS16**

(b) **ICCSS17**

FIG. 8. **Contact matrices for country of residence.** We compute for each conference the contact matrix in connectivity (*i.e.* link density) and interactivity (*i.e.* average total contact duration) considering the country of residence (top row). We then test the statistical significance of the values of the contact matrices by performing three different null models: P[**k**] (Null model 1), P[$p(\mathbf{w})$] (Null model 2) and P[**iso**(**g**)] (Null model 3). Positive deviations are in red and negative deviations in blue. Deviations marked in white with a star are significant under $p < 0.01$ (taking into account a Bonferroni correction).

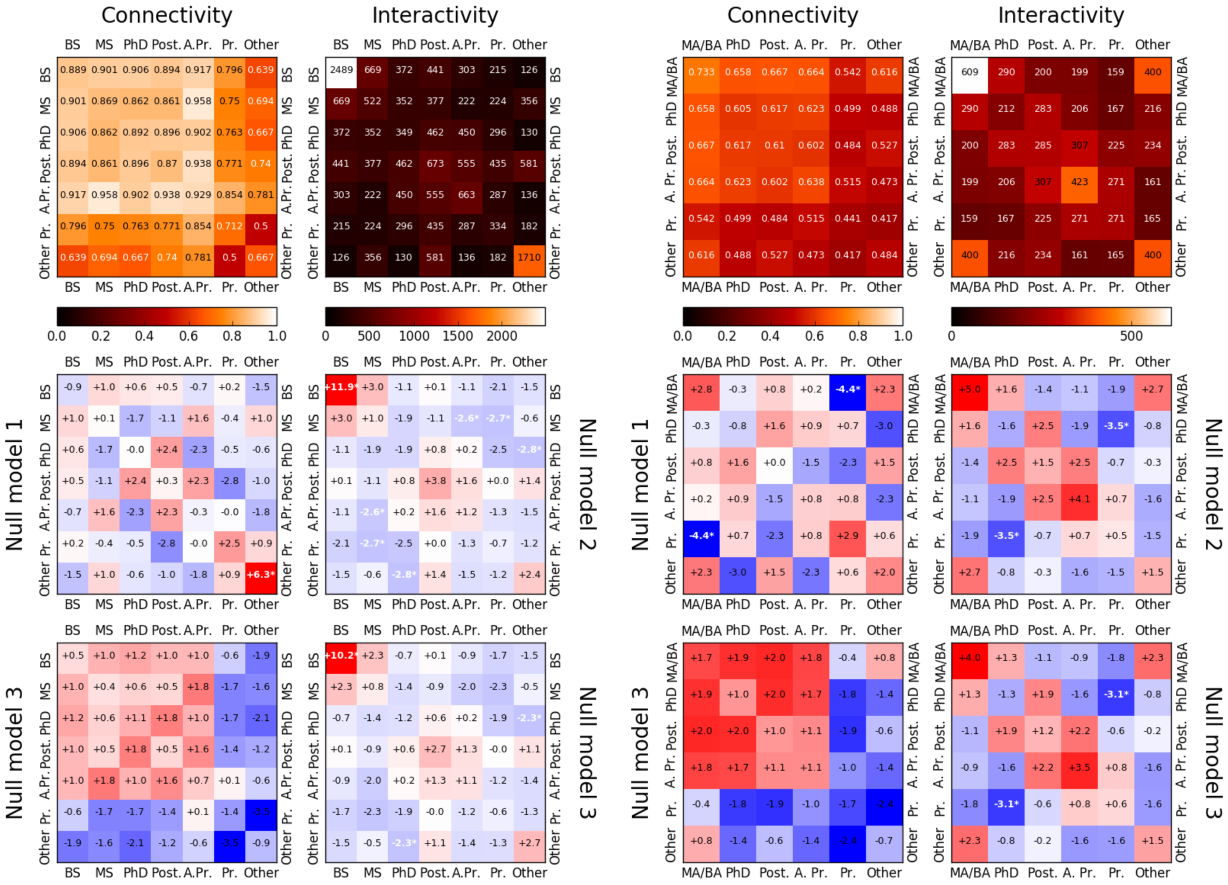

(a) **WS16** (b) **ICCSS17**

FIG. 9. **Contact matrices for academic status.** We compute for each conference the contact matrix in connectivity (*i.e.* link density) and interactivity (*i.e.* average total contact duration) considering the academic status (top row). We then test the statistical significance of the values of the contact matrices by performing three different null models: P[$\mathbf{k}$] (Null model 1), P[$p(\mathbf{w})$] (Null model 2) and P[$\mathbf{iso}(\mathbf{g})$] (Null model 3). Positive deviations are in red and negative deviations in blue. Deviations marked in white with a star are significant under $p < 0.01$ (taking into account a Bonferroni correction).

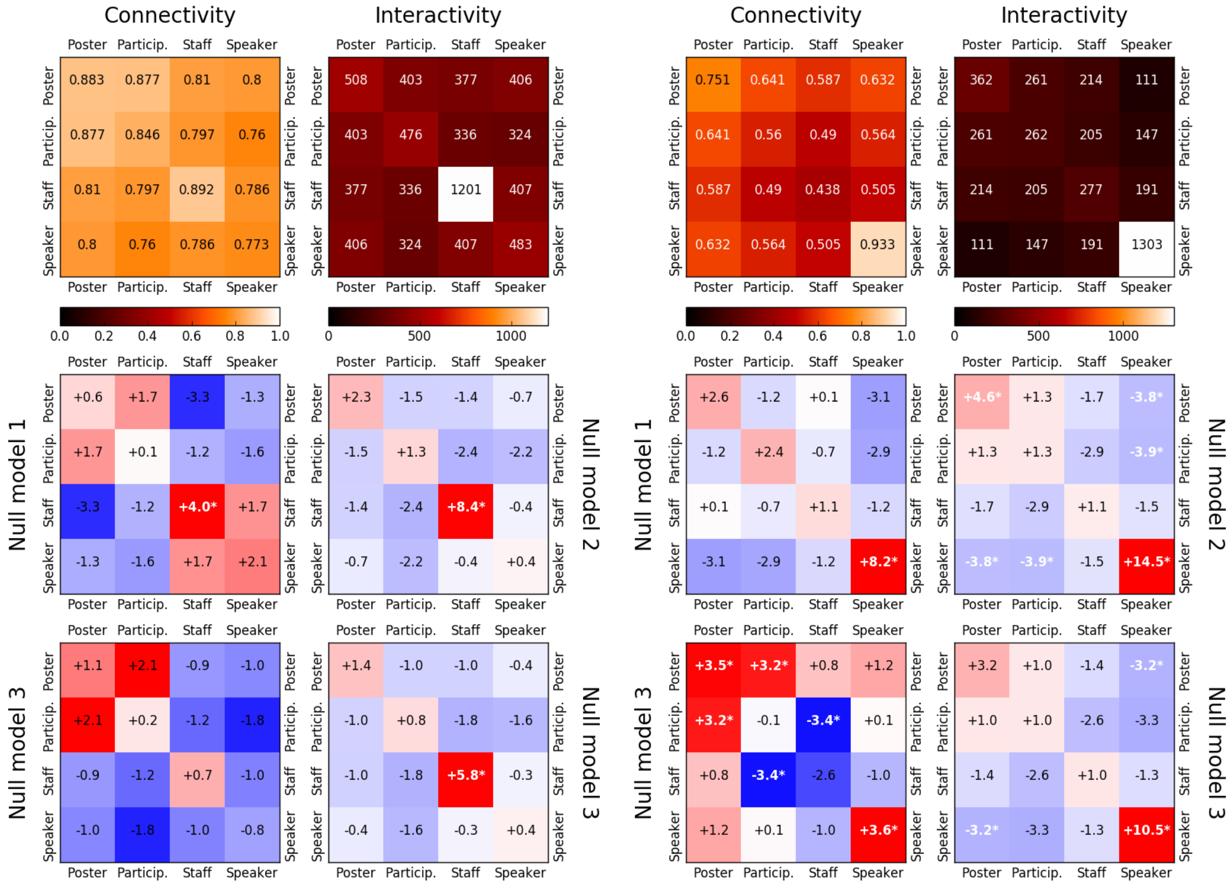


(a) **WS16**

(b) **ICCSS17**

FIG. 10. **Contact matrices for role in the conference.** We compute for each conference the contact matrix in connectivity (*i.e.* link density) and interactivity (*i.e.* average total contact duration) considering the role in the conference (top row). We then test the statistical significance of the values of the contact matrices by performing three different null models: P[$\mathbf{k}$] (Null model 1), P[$p(\mathbf{w})$] (Null model 2) and P[$\mathbf{iso}(\mathbf{g})$] (Null model 3). Positive deviations are in red and negative deviations in blue. Deviations marked in white with a star are significant under $p < 0.01$ (taking into account a Bonferroni correction).

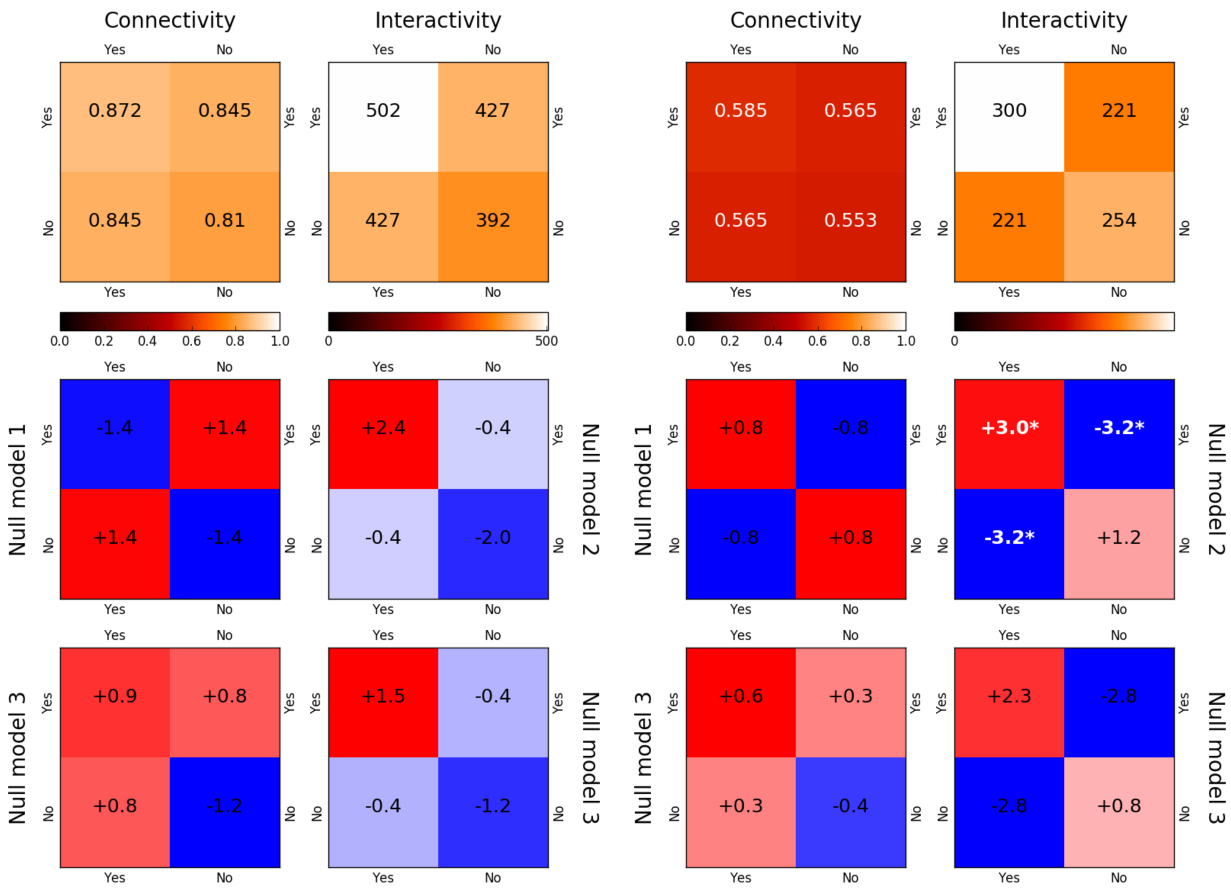


(a) **WS16**

(b) **ICCSS17**

FIG. 11. **Contact matrices for previus participation.** We compute for each conference the contact matrix in connectivity (*i.e.* link density) and interactivity (*i.e.* average total contact duration) considering the previous participation (top row). We then test the statistical significance of the values of the contact matrices by performing three different null models: P[$\mathbf{k}$] (Null model 1), P[$p(\mathbf{w})$] (Null model 2) and P[$\mathbf{iso}(\mathbf{g})$] (Null model 3). Positive deviations are in red and negative deviations in blue. Deviations marked in white with a star are significant under $p < 0.01$ (taking into account a Bonferroni correction).

| | WS16 | | | | ICCSS17 | | | |
|---|---|---|---|---|---|---|---|---|
| | $P[\mathbf{k}]$ | $P[\mathbf{iso}(\mathbf{g})]$ $(k)$ | $P[p(\mathbf{w})]$ | $P[\mathbf{iso}(\mathbf{g})]$ $(w)$ | $P[\mathbf{k}]$ | $P[\mathbf{iso}(\mathbf{g})]$ $(k)$ | $P[p(\mathbf{w})]$ | $P[\mathbf{iso}(\mathbf{g})]$ $(w)$ |
| Age | + 30-40 | (+ <30)<br>(+ 30-40)<br>(− >40) | + <30<br>− >40 | + <30<br>− >40 | + 40-49↔>50<br>− 40-49 | | + 30-39<br>− <30↔>50 | |
| Gender | | | + M | | + F<br>− M | | | |
| Country | | | + Other<br>− C1↔Other | + Other<br>− C1↔Other | + C1<br>+ C2<br>+ C4<br>− C1↔C2<br>− C1↔Other | + C3 | + C1<br>+ C2<br>(+ C3)<br>(+ C4)<br>(+ Other)<br>− C1↔C2<br>− C1↔C4<br>− C1↔Other<br>− C2↔C4<br>− C2↔Other | + C1<br>(+ C2)<br>(+ C3)<br>(+ C4)<br>− C1↔C2<br>(− C1↔C4) |
| Language | + L1 | (− L1↔Other) | + L2<br>− L1↔Other | + L2<br>− L1↔Other | + L4<br>(+ L3)<br>− L1↔L4 | | + L1<br>+ L2<br>+ L4<br>(+ L5)<br>− L1↔L2<br>− L1↔L4<br>− L4↔L5 | + L1<br>(+ L2)<br>(+ L3)<br>(+ L4)<br>(+ L5)<br>− L1↔L4<br>(− L1↔L2) |
| Academic status | + Other | (− Pr↔Other) | + BS<br>(+ Postdoc)<br>− MS↔A.Pr.<br>− MS↔Pr.<br>− PhD↔Other | + BS<br>− PhD↔Other | − MA/BA↔Pr.<br>(− PhD↔Other) | | (+ MA/BA)<br>(+ A.Pr.)<br>− PhD↔Pr. | (+ MA/BA)<br>(+ A.Pr.)<br>− PhD↔Pr. |
| Discipline | + Comp.Sc.↔Ph/M<br>(− Soc.Sc.↔Comp.Sc.) | | + Soc.Sc.<br>(− Soc.Sc.↔Comp.Sc.) | +Soc.Sc. | + CS<br>− CS↔SPB | | + CS<br>(+ MCL)<br>− SPB↔Other | + CS<br>(+ MCL) |
| Role | + Staff<br>(− Poster↔Staff) | | +Staff | +Staff | + Speaker<br>(− Poster↔Speaker) | + Poster<br>+ Poster↔Partic.<br>+ Speaker<br>− Partic.↔Speaker | + Poster<br>+ Speaker<br>− Poster↔Speaker<br>− Partic.↔Speaker | + Speaker<br>(+ Poster)<br>− Poster↔Speaker |
| Prev. Part. | | | | | | | + Yes<br>− Yes↔No | |

TABLE II. **Deviations from the null models.** We list per dataset and per null model the deviations fron the null models. Positive deviations are marked with a green plus (+), negative deviations with a red minus (−). Deviations that are larger than 3 sigmas but not significant under the $p < 0.01$ rule are marked with a $\sim$. Cases within a particular group are noted with the label of the group, cases between groups are noted with a ↔.

## V. LINK DYNAMICS

Table III reports the numbers used to draw the Figure 5 of the main text. Figures 12, 13, 14 show the contact matrices considering only links that are both conserved and reinforced between two consecutive days.

| | **WS16** | | **ICCSS17** | | |
|---|---|---|---|---|---|
| Day | 1 | 2 | 1 | 2 | 3 |
| Edges | 6681 | 3858 | 11125 | 9359 | 3602 |
| Node loss | 1987 | 0 | 1870 | 3603 | 0 |
| Node gain | 0 | 372 | 0 | 966 | 581 |
| Link loss | 1652 | 0 | 4963 | 4008 | 0 |
| Link gain | 0 | 444 | 0 | 4101 | 1273 |
| Conserved | 3042 | 0 | 4292 | 1748 | 0 |

TABLE III. **Link flows numbers.** For each pair of consecutive days in both conferences, we report the total number of edges, and the number of edges in each flow.

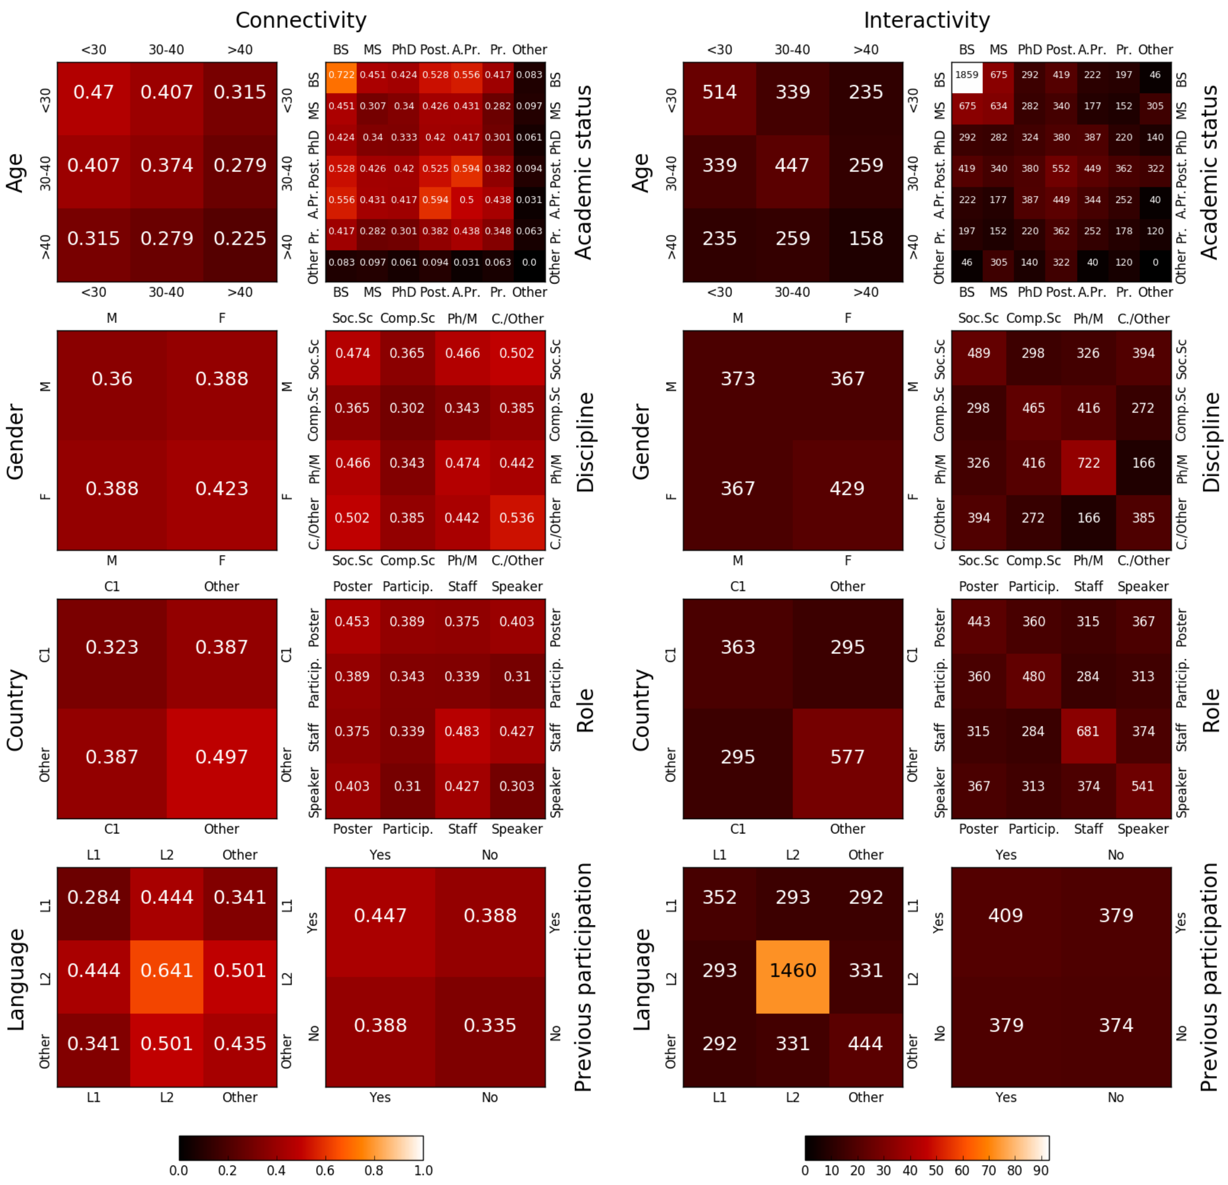


(a) **Connectivity** (b) **Interactivity**

FIG. 12. **Connectivity matrices - Filtered links — WS16, Day 1 → Day 2.**

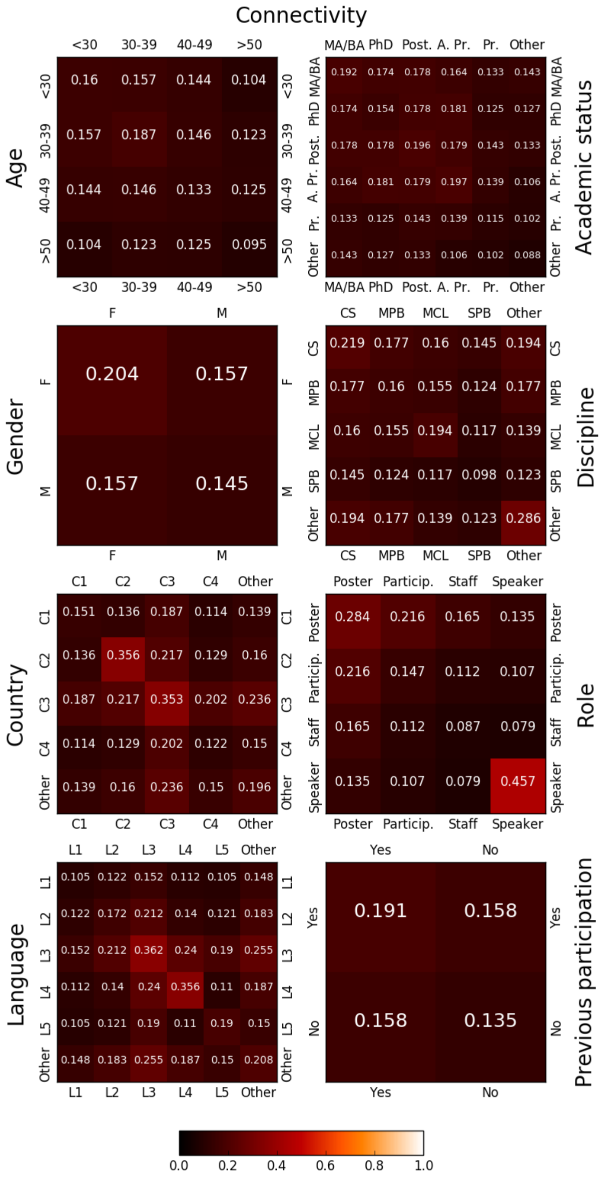


(a) **Connectivity**

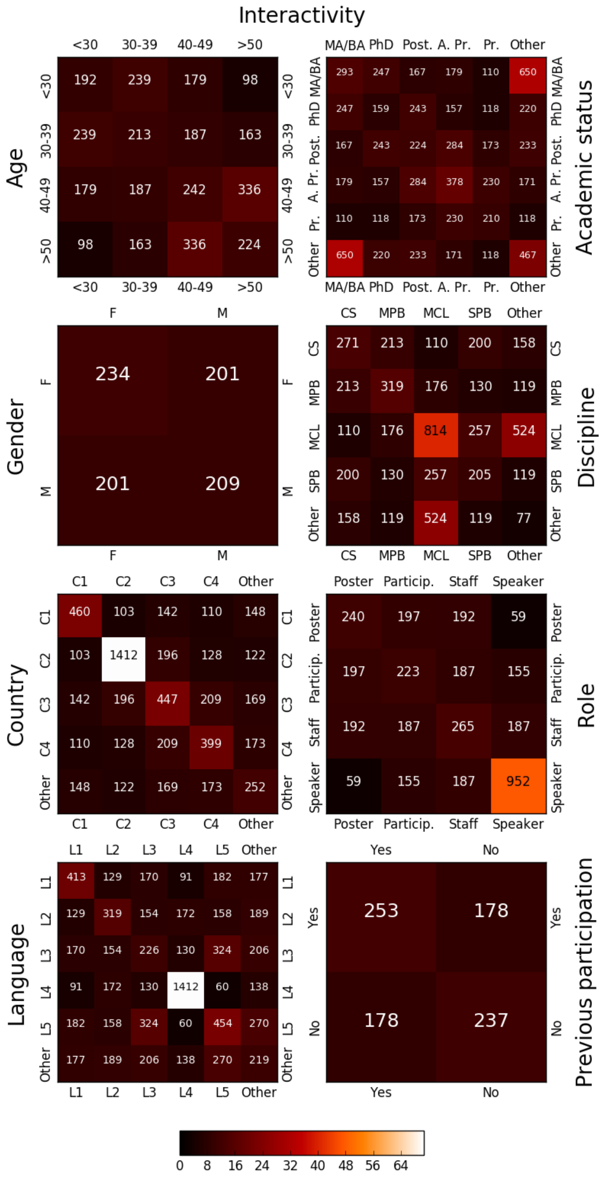


(b) **Interactivity**

FIG. 13. **Connectivity matrices - Filtered links — ICCSS17, Day 1 → Day 2.**

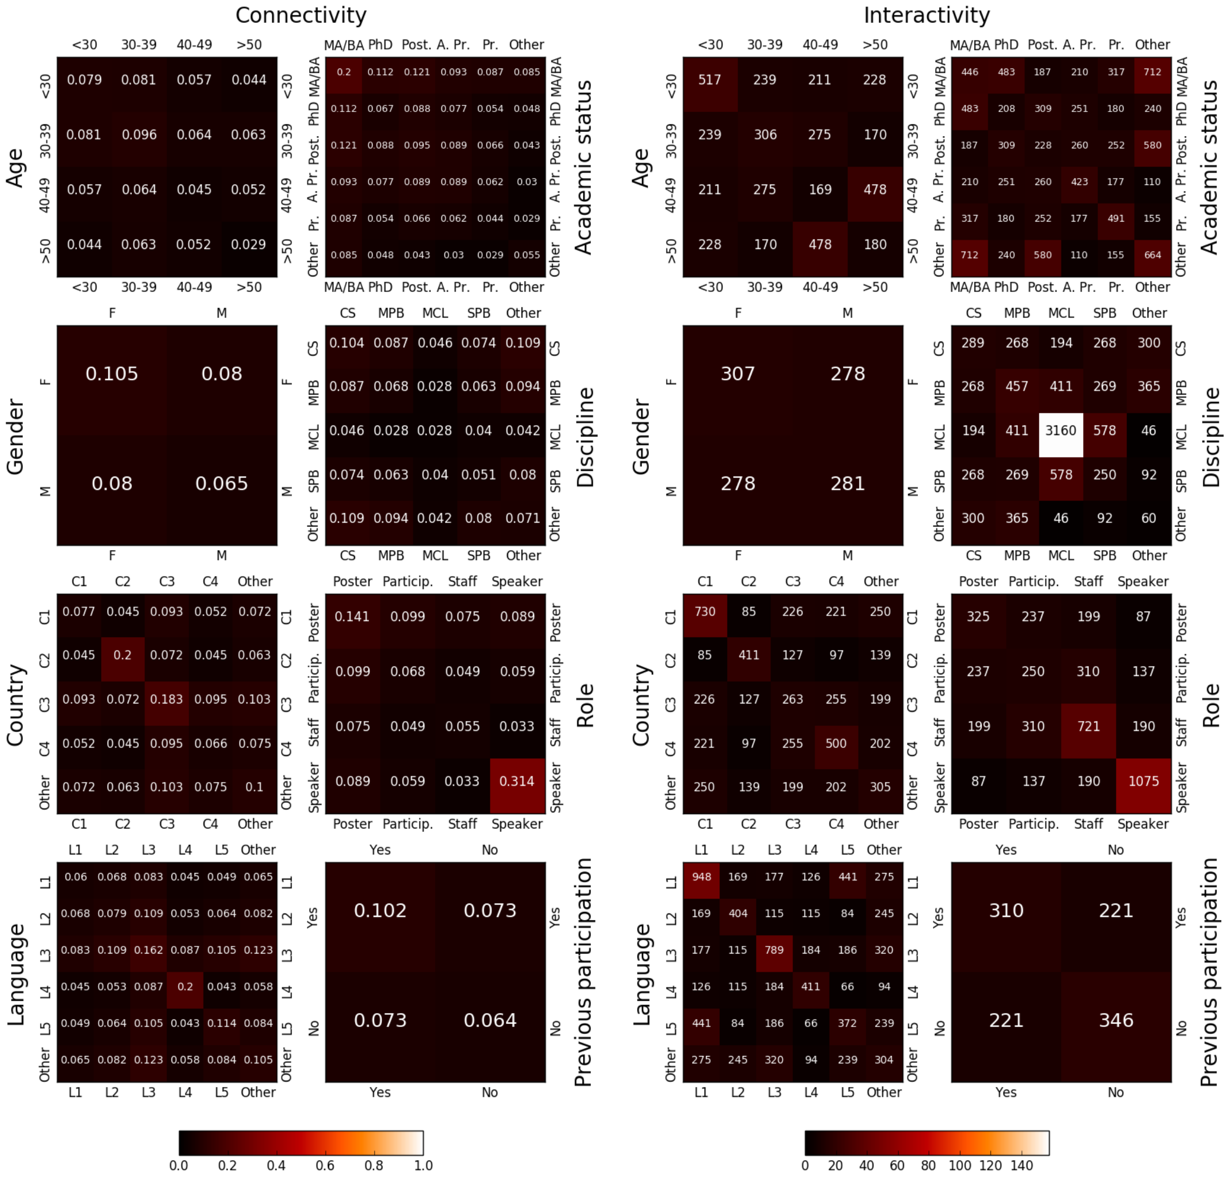


(a) **Connectivity**

(b) **Interactivity**

FIG. 14. **Connectivity matrices - Filtered links — ICCSS17, Day 2 → Day 3.**
